# Supplementary material for: Design and Performance of Parallel-channel Nanocryotrons in Magnetic Fields
Source: arXiv:2310.06108 source file (2023-12-04)
Supplement: Supplementary file 1 [file SM-APL.pdf]

# Supporting Information

## Design and Performance of Parallel-channel Nanocryotrons in Magnetic Fields

*Timothy Draher[1,2], Tomas Polakovic[3], Yi Li[1], John Pearson[1,4], Alan Dibos[1,4], Zein-Eddine Meziani[3], Zhili Xiao[1,2], Valentine Novosad[1,a]*

[1] Argonne National Laboratory, Materials Science Division, Lemont Illinois, 60439, USA.

[2] Northern Illinois University, Department of Physics, Dekalb Illinois, 60115, USA

[3] Argonne National Laboratory, Physics Division, Lemont Illinois, 60439, USA

[4] Center for Nanoscale Materials, Argonne National Laboratory, Argonne, IL 60439,

[a] Authors to whom correspondence should be addressed: Valentine Novosad, Email: novosad@anl.gov;

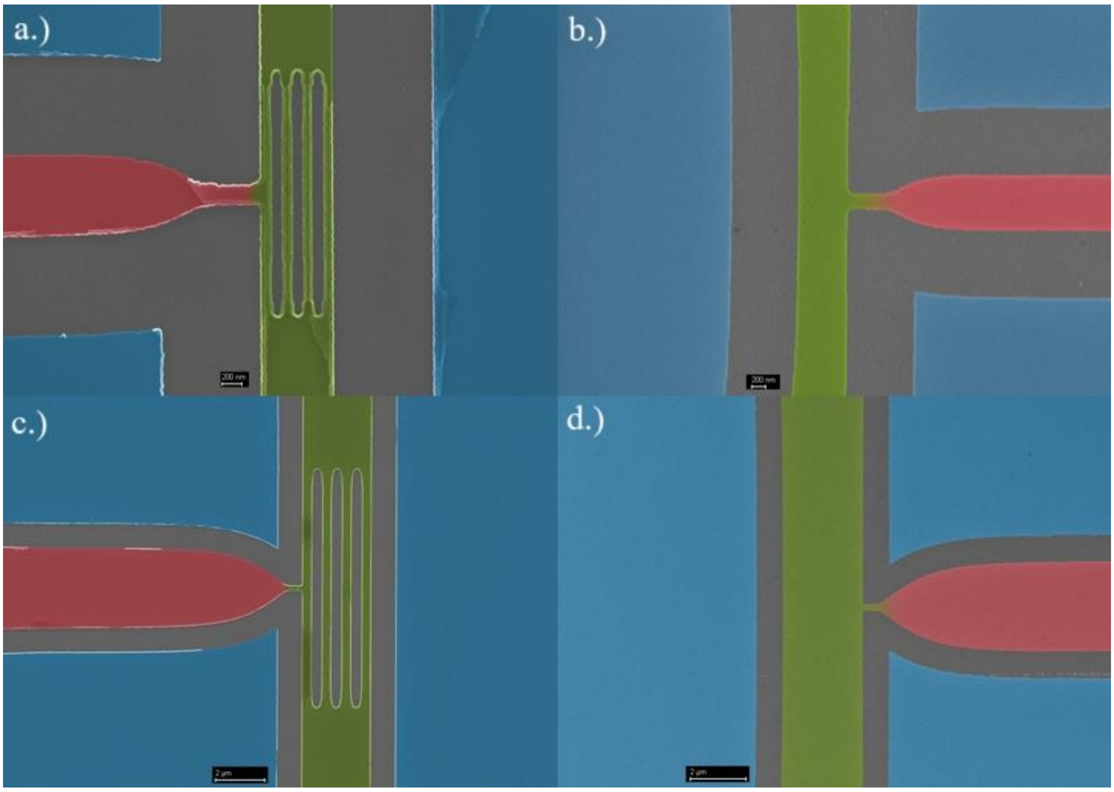


**Figure S1.** Colorized SEM images: 1:2 parallel-channel nTron (a.), 1:2 conventional nTron (b.), 1:8 parallel-channel nTron (c.), and 1:8 conventional nTron (d.). Blue highlights the ground plane, grey shows the trench and nanowire gaps, green represents the effective NbN channel, and red signifies the NbN gate to choke constriction. Scale bars correspond to 200 nm and 2 µm for both geometries, respectively.

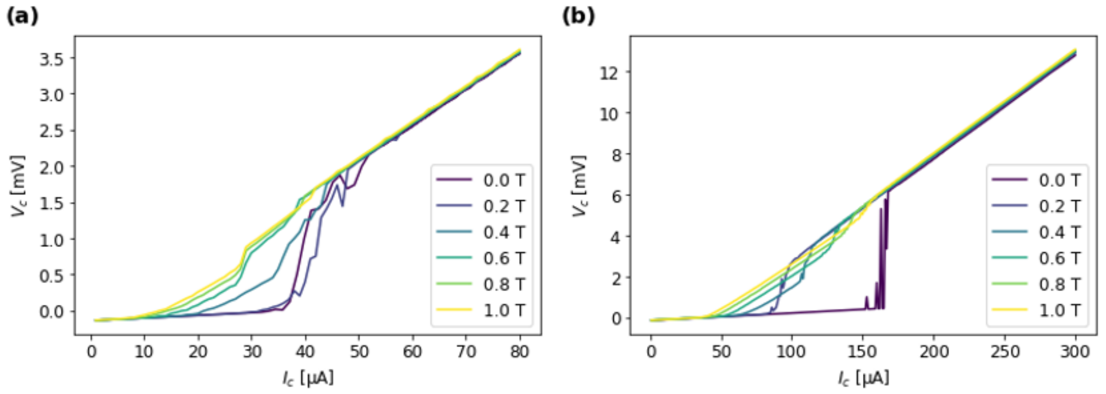


**Figure S2.** Parallel-channel nTron channel scans for $H_z$ up to 1 Tesla. 1:2 nTron (a) and 1:8 nTron (b) are shown. Due to the stochastic nature of the 1:8 device at 0 T, a curve close to the average $I_c^{channel}$ is shown.

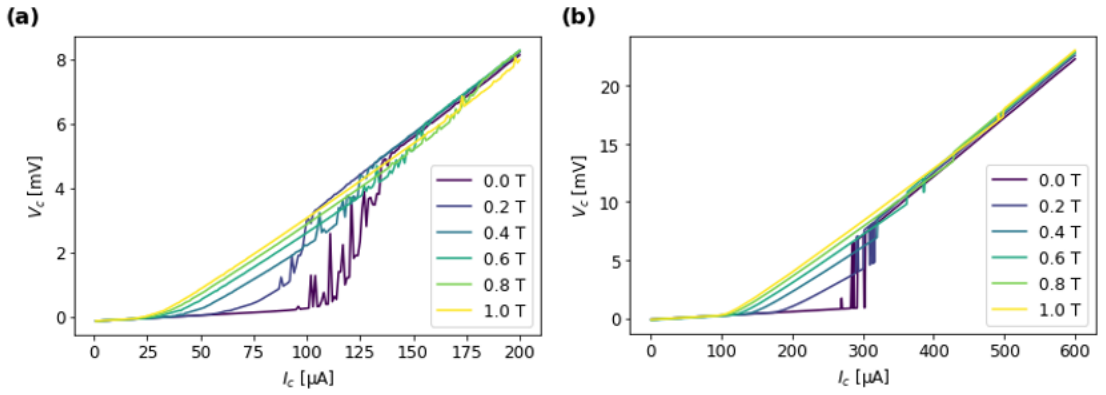


**Figure S3.** Conventional nTron channel scans for $H_z$ up to 1 Tesla. 1:2 nTron (a) and 1:8 nTron (b) are shown. Due to the stochastic nature of the 1:8 device at 0 and 0.2 T, curves close to the average $I_c^{channel}$ are shown.

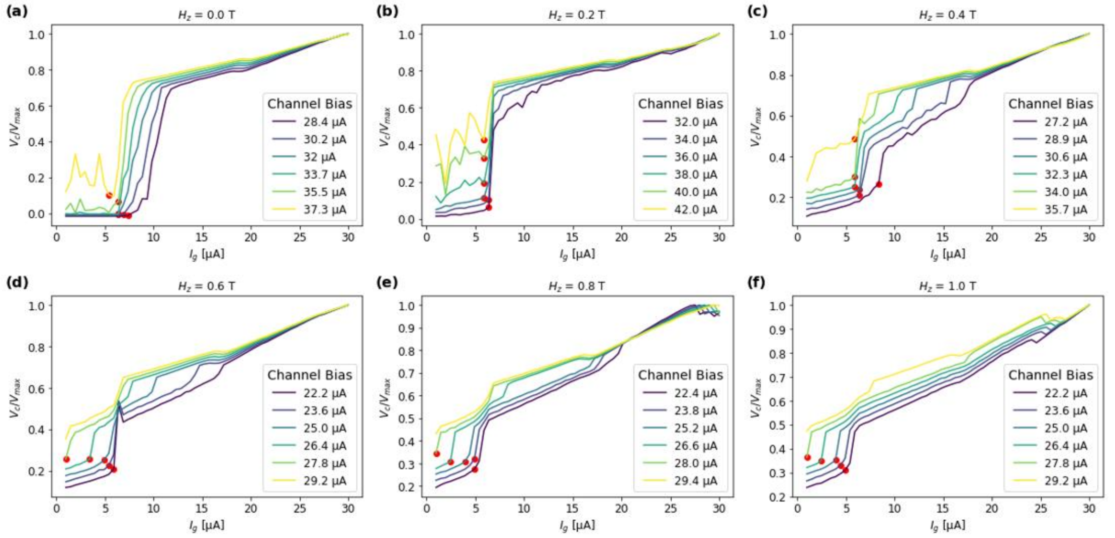


**Figure S4.** Normalized 1:2 parallel-channel nTron gate scans for $H_z$ up to 1 Tesla (a-f). Channel bias is set iteratively from 0.80-1.05 $I_c^{channel}$ and red points signify the critical gate current $I_c^{gate}$ at a given bias.

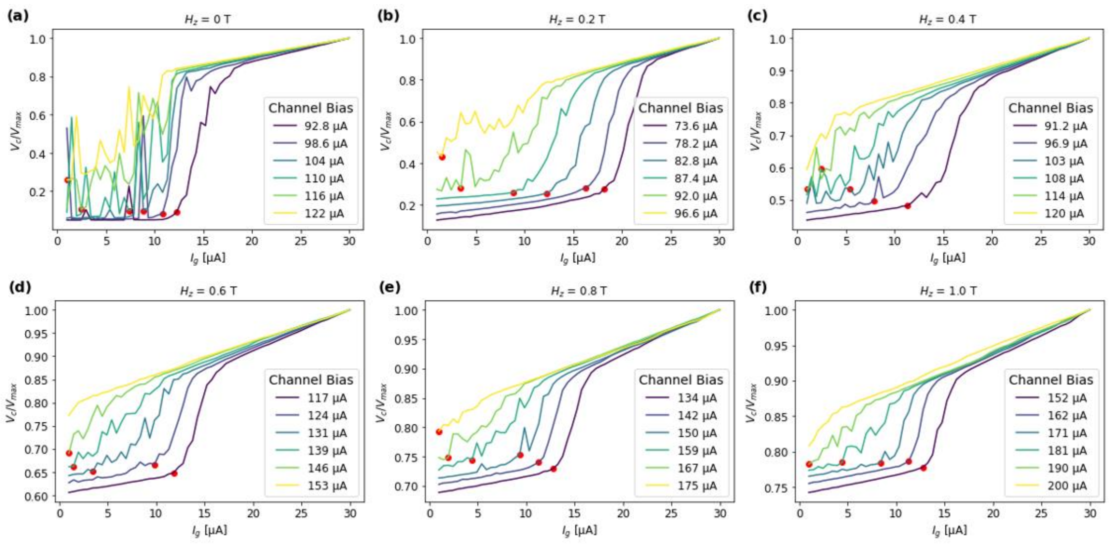


**Figure S5.** Normalized 1:2 conventional nTron gate scans for $H_z$ up to 1 Tesla (a-f). Channel bias is set iteratively from 0.80-1.05 $I_c^{channel}$ and red points signify the critical gate current $I_c^{gate}$ at a given bias.

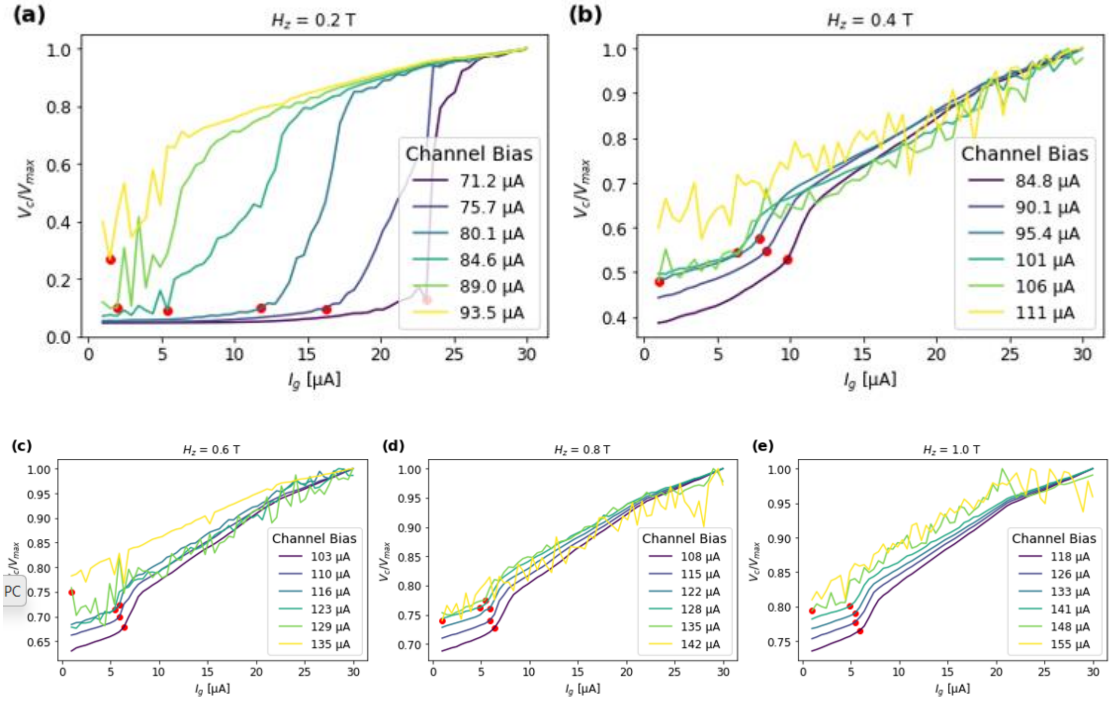


**Figure S6.** Normalized 1:8 parallel-channel nTron gate scans for $H_z$ = 0.2 to 1 Tesla (a-e). Channel bias is set iteratively from 0.80-1.05 $I_c^{channel}$ and red points signify the critical gate current $I_c^{gate}$ at a given bias.

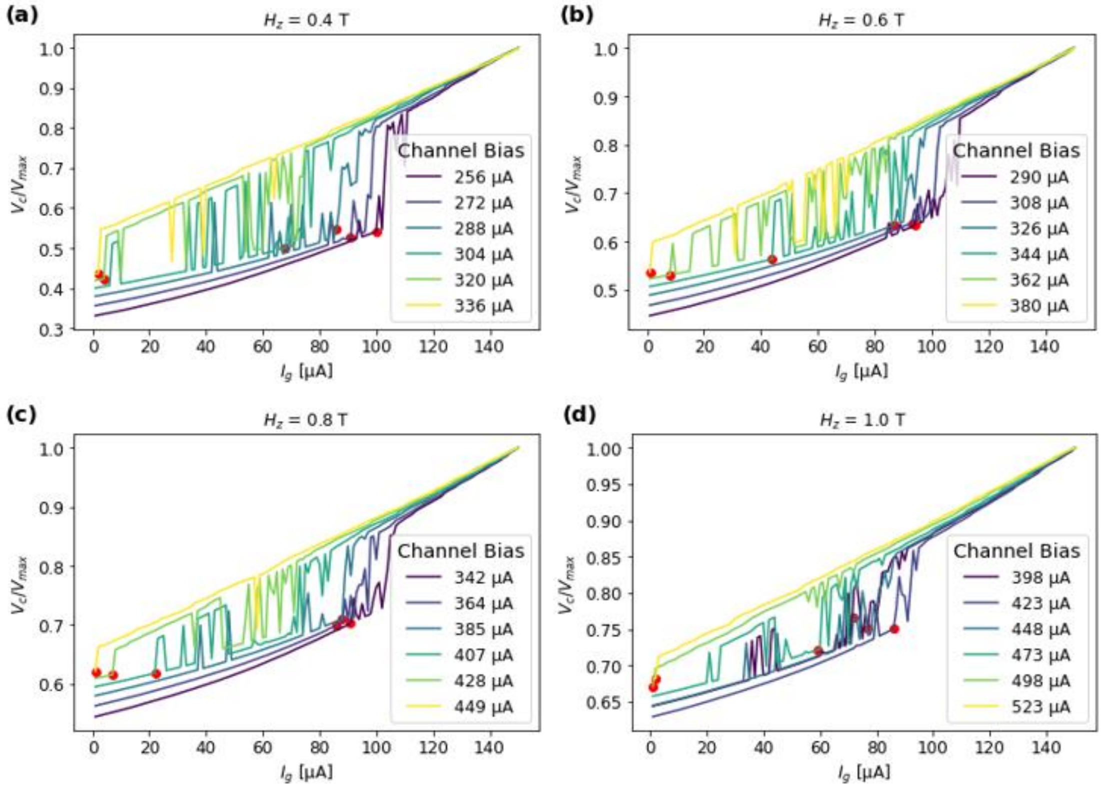


**Figure S7.** Normalized 1:8 conventional nTron gate scans for $H_z$ = 0.4 to 1 Tesla (a-d). Channel bias is set iteratively from 0.80-1.05 $I_c^{channel}$ and red points signify the critical gate current $I_c^{gate}$ at a given bias.

DC Gate Characterizations: The nTron channels were screened with current until a sharp voltage transition is observed, indicating the nTron switching into the fully resistive state. Once $I_c^{channel}$ is known, the channel is biased iteratively at 0.80-1.05 $I_c^{channel}$ and current is scanned through the gate. Fig. S2-3 display the channel scans and Fig. S4-7 show the gate scans for all island and conventional 1:2 and 1:8 nTron ratios, respectively. Red dots indicate $I_c^{gate}$, where the hot spot forms within the choke. $I_c^{gate}$ was determined using a local 10% voltage threshold to screen out voltage oscillations caused by vortex crossings and to emphasize the full transition rather than intermediate states. If a given gate scan begins already in the resistive state given by a high bias (i.e. often at 1.05 $I_c^{channel}$), $I_c^{gate}$ is then set to zero. Consequently, if a given gate scan begins in the midst of a transition (i.e. often at or near 1.0 $I_c^{channel}$), $I_c^{gate}$ is then fixed to 1 μA. The 1:8 parallel channel nTron shows stochastic switching behavior

for a window of $I_c^{channel}$, at $H_z = 0$ T and $H_z =$ 0 and 0.2 T for the 1:8 conventional nTron. Thus, at these field environments gate scans were swept iteratively fifty times to build a statistical distribution of the average of $I_c^{gate}$ and its standard deviation. Hence the switching characteristic diagrams in Figures 2-3 represent the average of $I_c^{gate}$ and error bars denoting one standard deviation. Tables S1-S3 show the statistical values extracted for the 1:8 devices in the given stochastic $H_z$ environment.

| Channel Bias (μA) | Avg. $I_c^{gate}$ (μA) | Std. Deviation σ (μA) |
|---|---|---|
| 134 (0.80 $I_c^{channel}$) | 29.0 | 0.68 |
| 143 (0.85 $I_c^{channel}$) | 25.5 | 0.90 |
| 151 (0.90 $I_c^{channel}$) | 24.5 | 1.18 |
| 160 (0.95 $I_c^{channel}$) | 20.3 | 3.10 |
| 168 (1.00 $I_c^{channel}$) | 8.33 | 4.00 |
| 176 (1.05 $I_c^{channel}$) | 9.22 | 0.00 |

**Table S1.** Summary of 1:8 parallel-channel nTron stochastic gate scan statistics at $H_z = 0$ T.

| Channel Bias (μA) | Avg. $I_c^{gate}$ (μA) | Std. Deviation σ (μA) |
|---|---|---|
| 234 (0.80 $I_c^{channel}$) | 100 | 2.75 |
| 248 (0.85 $I_c^{channel}$) | 86.2 | 6.52 |
| 263 (0.90 $I_c^{channel}$) | 62.6 | 11.2 |
| 277 (0.95 $I_c^{channel}$) | 34.8 | 17.3 |
| 292 (1.00 $I_c^{channel}$) | 28.1 | 16.1 |
| 307 (1.05 $I_c^{channel}$) | 15.7 | 11.3 |

**Table S2.** Summary of 1:8 conventional nTron stochastic gate scan statistics at $H_z =$ 0 Tesla.

| Channel Bias (μA) | Avg. $I_c^{gate}$ (μA) | Std. Deviation σ (μA) |
|---|---|---|
| 238 (0.80 $I_c^{channel}$) | 93.6 | 2.22 |
| 253 (0.85 $I_c^{channel}$) | 86.3 | 4.94 |
| 262 (0.90 $I_c^{channel}$) | 75.1 | 9.16 |
| 283 (0.95 $I_c^{channel}$) | 41.9 | 14.5 |
| 298 (1.00 $I_c^{channel}$) | 29.6 | 12.6 |
| 313 (1.05 $I_c^{channel}$) | 16.8 | 14.1 |

**Table S3.** Summary of 1:8 conventional nTron stochastic gate scan statistics at $H_z$ = 0.2 T.

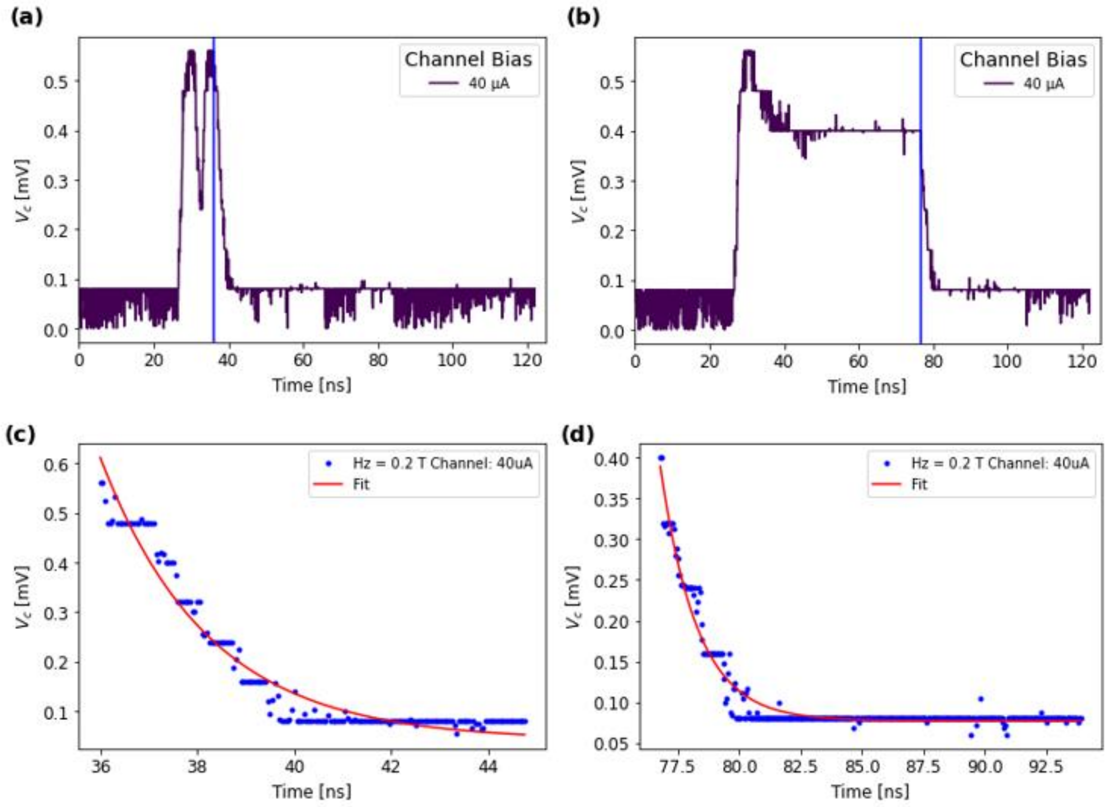


**Figure S8.** Examples of double pulse (a) and step response pulse (b) for the 1:2 parallel-channel nTron device. Blue vertical lines mark the voltage signal peak before decay. Corresponding exponential decay fits for τ extraction are shown: double pulse (c) and step response (d).

| Device | Voltage (V) | Duration (ns) | Delay (ns) | Attenuation (dB) |
|---|---|---|---|---|
| 1:2 Gapped nTron | 4.5 | 4.4 | 6 | 20 |
| 1:8 Gapped nTron | 4.5 | 4.4 | 6 | 13 |
| 1:2 Conv. nTron | 4.5 | 3 | 4 | 20 |
| 1:8 Conv. nTron | 4.8 | 4 | 7 | 14 |

**Table S4.** Pulse parameters for nTron devices at all $H_z$. Duration and delay apply only to the double pulse technique. Step response pulse duration is fixed at 50 ns. Field environments that promote probabalistic behavior and required variable attenuation for the 1:8 designs are omitted and shown in Table S5.

| Channel Bias (μA) $H_z = 0\ T$ | Attenuation (dB) |
|---|---|
| 134 (0.80 $I_c^{channel}$) | 11 |
| 143 (0.85 $I_c^{channel}$) | 11 |
| 151 (0.90 $I_c^{channel}$) | 11 |
| 160 (0.95 $I_c^{channel}$) | 12 |
| 168 (1.00 $I_c^{channel}$) | 12 |

| Channel Bias (μA) $H_z = 0\ T$ | Attenuation (dB) |
|---|---|
| 234 (0.80 $I_c^{channel}$) | 12 |
| 248 (0.85 $I_c^{channel}$) | 13 |
| 263 (0.90 $I_c^{channel}$) | 13 |
| 277 (0.95 $I_c^{channel}$) | 14 |
| 292 (1.00 $I_c^{channel}$) | 14 |

**Table S5.** Pulse attenuation for 1:8 parallel-channel nTron at $H_z = 0$ T (left) and 1:8 conventional nTron (right).
